# Supplementary material for: Recurrent Feedback Improves Feedforward Representations in Deep Neural Networks
Source: arXiv:1912.10489 source file (2019-12-22)
Supplement: Supplementary file 1 [file supplementary.tex]

\section{Supplementary Materials}

\subsection{Details of different contextual modules}

We tested three other possible contextual modules in Section~\ref{sec:exps_and_analysis}. Here are the detailed formulations of the three modules.

\begin{subequations}
\label{eqs:gate1}
\begin{align}
O_{k}^{(t)} & = gate * contextual + O_{k}^{(t-1)}\\
gate &= \NNTanh(\NNConv_{1\times1}(\NNUpsample(O_{h(k)}^{(t-1)}))) \\
contextual &= \NNConv_{3\times3}(\NNConcat(\NNUpsample(O_{h(k)}^{(t-1)}), O_{k-1}^{(t-1)}))
\end{align}
\end{subequations}

\begin{subequations}
\label{eqs:gate2}
\begin{align}
O_{k}^{(t)} &= gate * contextual + O_{k}^{(t-1)}\\
gate &= \NNTanh(\NNConv_{1\times1}(\NNConcat(\NNUpsample(O_{h(k)}^{(t-1)}), O_{k-1}^{(t-1)}))) \\
contextual &= \NNConv_{3\times3}(\NNConcat(\NNUpsample(O_{h(k)}^{(t-1)}), O_{k-1}^{(t-1)}))
\end{align}
\end{subequations}

\begin{subequations}
\label{eqs:gate3}
\begin{align}
O_{k}^{(t)} & = gate\_contextual * O_{k+h(k)}^{(t-1)} + gate * contextual + O_{k}^{(t-1)}\\
gate & = \NNTanh(\NNConv_{1\times1}(\NNUpsample(O_{h(k)}^{(t-1)}))) \\
contextual  & = \NNConv_{3\times3}(\NNConcat(\NNUpsample(O_{h(k)}^{(t-1)}), O_{k}^{(t-1)})) \\
gate\_contextual &= \NNTanh(contextual)
\end{align}
\end{subequations}

In the module described by Eqs.~\eqref{eqs:gate1}, we first generated the gate by the top-down layer. Then we used the gate to control the contextual information generated by concatenating bottom-up layer and top-down layer. To stable the information flow, we added it with the bottom-up layer.

In the module described by Eqs.~\eqref{eqs:gate2}, we first generated the gate by contextual information which is the same as our proposed module. Then we used the gate to control the contextual information itself which we thought was a feasible way to store the largest information. To stable the information flow, we also added it with the bottom-up layer.

We generated two gates by both contextual information and top-down layer in the module described by Eqs.~\eqref{eqs:gate3}. Then we used the gate\_contextual to control the top-down information and used the gate to control the contextual information. To stable the information flow, we also added it with the bottom-up layer.

\subsection{Image Examples of Different Tasks}
In this section, we showed some examples of image occlusion task and adversarial noise task.

In the left of Figure~\ref{fig:occlusion-adver}, we showed one image occlusion example. And we showed one adversarial noise example in the right of Figure~\ref{fig:occlusion-adver}.

\begin{figure}
\centering
\begin{minipage}[c]{0.48\textwidth}
\centering
\includegraphics[width=6cm]{Figures/occlusion.png}
\label{fig:sparsity}
\end{minipage}
\begin{minipage}[c]{0.48\textwidth}
\centering
\includegraphics[width=6cm]{Figures/fish.png}
\caption{Examples of different task. \textbf{Left}: An example of image occlusion task. We quantified the scale of occluders in the image. \textbf{Right}: An example of Adversarial Attack noise. We can see the noise is not obvious to the human eyes but can lead a significant influence to the neural network. We used Fast Gradient Sign Non-target to generate the noise. The left is the original image and the right one is the image adding the noise.}
\label{fig:occlusion-adver}
\end{minipage}
\end{figure}

\begin{table*}
\capbtabbox{
  \begin{tabular}{l|c|c|c|c|c|c}
  \toprule
  \cmidrule(r){1-2}
  \diagbox{Noise Level}{Models} & VGG16 & VGG-LR-2 & VGG-GCM-4\\
  \midrule
  0 & 71.076 & 71.551 & \textbf{71.741} \\
  10 & 65.456 & 66.012 & \textbf{67.620} \\
  20 & 54.090 & 54.640 & \textbf{56.988} \\
  30 & 39.124 & 39.634 & \textbf{43.686} \\
  40 & 24.068 & 24.721 & \textbf{29.120} \\
  50 & 13.072 & 13.907 & \textbf{18.202} \\
  \bottomrule
  \end{tabular}
}{
 \caption{Noise image classification top-1 accuracy on Imagenet.}
 \label{tab:noise-imn-top1}
}
\end{table*}

\subsection{ImageNet Top1 Accuracy}

In Table ~\ref{tab:imagenet-top1}, we showed the Imagenet Top1 accuracy results. Notice that we did not compare our model with VGG-ATT model proposed in \citep{jetley2018learn} because their model is not reasonable on high resolution image dataset. Therefore, their model cannot extract effective attention map from the ImageNet images.

\subsection{Noise ImageNet Top1 Accuracy}

In Table ~\ref{tab:noise-imn-top1}, we showed the Imagenet Top1 accuracy results with different level of Gaussian noise. VGG16 here means the standard VGG16 model. Notice that we also compared our model with \citep{li2018learning}'s model which we name "VGG-LR-4".
